# Supplementary material for: Grounded Language-Image Pre-training
Source: arXiv:2112.03857 source file (2022-06-17)
Supplement: Supplementary file 1 [file appendix.tex]

% CVPR 2022 Paper Template
% based on the CVPR template provided by Ming-Ming Cheng (https://github.com/MCG-NKU/CVPR_Template)
% modified and extended by Stefan Roth (stefan.roth@NOSPAMtu-darmstadt.de)

\documentclass[10pt,twocolumn,letterpaper]{article}

%%%%%%%%% PAPER TYPE  - PLEASE UPDATE FOR FINAL VERSION
%\usepackage[review]{cvpr}      % To produce the REVIEW version
\usepackage{cvpr}              % To produce the CAMERA-READY version
%\usepackage[pagenumbers]{cvpr} % To force page numbers, e.g. for an arXiv version

% Include other packages here, before hyperref.
\usepackage{graphicx}
\usepackage{amsmath}
\usepackage{amssymb}
\usepackage{booktabs}
\usepackage{latexsym}

\usepackage{url}
\usepackage{booktabs}
\usepackage{multirow}
\usepackage{array, caption, floatrow, makecell, booktabs}
\usepackage{wrapfig}
\usepackage{floatrow}
\usepackage{comment}
\usepackage{enumitem}
\usepackage{accents}
%%%%%%%%%%%%%%%%%%%%%%%%%%%%%%%%%%%%%%%%%
\usepackage{xspace,mfirstuc,tabulary}
\usepackage{xcolor}
\usepackage[table]{xcolor}
\usepackage{colortbl}
\usepackage{tabu}
\usepackage{todonotes}
\makeatletter
\newcommand*\iftodonotes{\if@todonotes@disabled\expandafter\@secondoftwo\else\expandafter\@firstoftwo\fi}  % defines \iftodonotes{<true>}{<false>}, thanks to https://tex.stackexchange.com/questions/126559/conditional-based-on-packageoption
\makeatother

% Note that these macros accept optional arguments such as size=\small, bordercolor=red, and so on.  Capitalized versions are inline paragraphs instead of margin notes.
 % to mark stuff that you know is missing or wrong when you write the text
 % default note settings, used by macros below.

\usepackage{dingbat}
\usepackage{pifont}% http://ctan.org/pkg/pifont
%
%

% It is strongly recommended to use hyperref, especially for the review version.
% hyperref with option pagebackref eases the reviewers' job.
% Please disable hyperref *only* if you encounter grave issues, e.g. with the
% file validation for the camera-ready version.
%
% If you comment hyperref and then uncomment it, you should delete
% ReviewTempalte.aux before re-running LaTeX.
% (Or just hit 'q' on the first LaTeX run, let it finish, and you
%  should be clear).
\usepackage[pagebackref,breaklinks,colorlinks]{hyperref}

% Support for easy cross-referencing
\usepackage[capitalize]{cleveref}
\crefname{section}{Sec.}{Secs.}
\Crefname{section}{Section}{Sections}
\Crefname{table}{Table}{Tables}
\crefname{table}{Tab.}{Tabs.}

%%%%%%%%% PAPER ID  - PLEASE UPDATE
 % *** Enter the CVPR Paper ID here

\begin{document}

%%%%%%%%% TITLE - PLEASE UPDATE
\title{Appendix of Grounded Language-Image Pre-training
}

\maketitle

\definecolor{Graylight}{gray}{0.95}

\newcommand{\our}{GLIP\xspace}
\newcommand{\dyground}{ZS DyHead\xspace}
\newcommand{\ourtiny}{GLIP-Tiny\xspace}

\newcommand{\objfive}{Object365\xspace}

\newcommand{\oura}{GLIP$_\text{OD}$\xspace}
\newcommand{\ourb}{GLIP$_\text{Ground}$\xspace}
\newcommand{\ourc}{GLIP$_\text{Web}$\xspace}

\newcommand{\ourd}{GLIP+\xspace}
\newcommand{\ourlarge}{GLIP+\xspace}

% dataset names
\newcommand{\goldg}{GoldG\xspace}
\newcommand{\goldgfull}{GoldG+\xspace}
\newcommand{\websmall}{Web4M\xspace}
\newcommand{\weblarge}{Web24M\xspace}

\newcommand{\std}[1]{\tiny{$\pm$#1}}

\input{sections/5_appendix_for_all}

\newpage
{\small
\bibliographystyle{ieee_fullname}
\bibliography{egbib}
}

\end{document}
